# Supplementary material for: Img-Diff: Contrastive Data Synthesis for Multimodal Large Language Models
Source: arXiv:2408.04594 source file (2024-12-19)
Supplement: Supplementary file 1 [file appendix_sota_mllms_compare.tex]

% Please add the following required packages to your document preamble:
% \usepackage{booktabs}
% \usepackage{graphicx}
\begin{table}[t]
\centering
\caption{}
\label{tab:sota_mllms_compare}
\resizebox{\columnwidth}{!}{%
\begin{tabular}{@{}ccccccccc@{}}
\toprule
Model                      & VQA$^{v2}$ & GQA  & POPE & MMB  & MMB$^{CN}$ & MM-Vet & SQA$^{I}$ & SEED \\ \midrule
BLIP-2 (13B)               & 41.0       & 41.0 & 85.3 & -    & -          & 22.4   & 61.0      & 46.4 \\
InstructBLIP (13B)         & 75.3       & 49.5 & 78.9 & 34.5 & 15.5       & 25.6   & 63.1      & 43.6 \\
Qwen-VL (7B)               & 78.8       & 59.3 & 78.1 & 38.2 & 7.4        & 38.2   & 67.1      & 56.3 \\
Qwen-VL-Chat (7B)          & 78.2       & 57.5 & 79.2 & 60.6 & 56.7       & 41.5   & 68.2      & 58.2 \\
SPHINX (13B)               & 78.1       & 62.6 & 80.7 & 66.9 & 56.2       & 36.0   & 69.3      & 69.1 \\ \midrule
LLaVA-1.5-7B               & 78.5       & 62.0 & 85.9 & 64.3 & 58.3       & 30.5   & 66.8      & 58.6 \\
\textbf{LLaVA-1.5-7B + RP} & 79.3       & 62.8 & 86.4 & 66.1 & 59.8       & 33.2   & 68.2      & 61.7 \\ \midrule
MGM-7B                     & 80.4       & 62.6 & 86   & 69.3 & 58.9       & 40.8   & 70.6      & 63.5 \\
\textbf{MGM-7B + RP}       & 80.7       & 62.7 & 86.2 & 68.7 & 59.6       & 44.1   & 71.7      & 63.2 \\ \midrule
InternVL2-8B-FT            & 81.8       & 62.6 & 87.7 & 82.5 & 81.5       & 49.2   & 96.5      & 69.5 \\
\textbf{InternVL2-8B + RP} & 81.8       & 62.6 & 88.0 & 82.7 & 81.4       & 52.6   & 96.6      & 69.9 \\ \bottomrule
\end{tabular}%
}
\end{table}
